# Supplementary material for: A Generic Top-N Recommendation Framework For Trading-off Accuracy, Novelty, and Coverage
Source: arXiv:1803.00146 source file (2018-03-01)
Supplement: Supplementary file 1 [file appendix-backup.tex]

\iffalse
\section{Results}
\subsection{Consumer Modelling} In this section, we look at the consumer modelling component of our work. 
Naturally, we expect users who rate more items to be more open to exploring unpopular items (higher risk-degree) and to have more varied tastes (lower focusing degree).  Figure~\ref{fig:analysisEstimates}.a plots the consumer modelling measures with respect to the the number of rated items. We observe that all risk measures, NorNLT, skewpop3, theta, thetaIDF, and thetaIDFN, are positively correlated with the number of rated items. Regarding the focusing degree, we observe that  as the users rate more movies, their average focusing degree decreases, which indicates that as users rate more and more items, they are  more likely to be rating diverse items.  \textcolor{red}{Can we also conclude that they have a higher desire for diversity? what about other datasets?} Moreover, the positive correlation  between risk-degrees and number of rated items also motivates using the  the number of items rated as a simple measure of risk. Figure~\ref{fig:analysisEstimates}.b  plots the average popularity of rated items   vs the number of rated items. We observe that as the number of rated items increases, their average popularity decreases.

 Figure~\ref{fig:analysisEstimates}.c shows the Pearson coefficient correlation matrix for  the ranked lists generated by  ordering the users by the various risk measures. The ranked list generated by ...

\begin{figure*}[htb]
\centering
\subfigure[Estimates vs \#rated items ]{
\includegraphics[width=0.25\textwidth]{Figures/general/oTrainNorNLTItemsoTrainSkewPop3thetathetaIDFNthetaIDFrhooveroTrainNRatings.pdf}}
\subfigure[popularity of rated items over n ratings]{
\includegraphics[width=0.25\textwidth]{Figures/general/popoveroTrainNRatings.pdf}}
\subfigure[coeff matrix]{
\includegraphics[width=0.29\textwidth]{Figures/Coeff/userOrderCoeffMatrix.pdf}}
\caption{analysis of estimated params}
\label{fig:analysisEstimates}
\end{figure*}
%However, as the user rate more items,  both skewness measures decrease, so they become more risk-averse which is wrong.  


Figure~\ref{fig:histograms} shows  the histograms of various consumer modelling measures (averaged across the users that fall in each bin).
Figure~\ref{fig:histograms}.b  shows the \# users vs number of long tail items rated (where the x-axis has been scaled to $[0,1]$ range). 
Figure~\ref{fig:histograms}.c shows the \# users vs normalized number of long tail items rated (equation~\ref{eq:NorNLT-risk} which has further been scaled to $[0,1]$ range).  
Figure~\ref{fig:histograms}.d shows the \# users vs number of items rated (where the x-axis has been scaled to $[0,1]$ range). 
This figure has a long tail distribution, which shows the majority of users rate a few items; therefore the number of ratings may  not distinguish between the users and will not serve as a good proxy of risk-degree.
Figure~\ref{fig:histograms}.e shows the histogram of focusing degree $\rho$ is normally distributed  across the users, with $\mu = 0.48$ and $\sigma = 0.14$. Thus, considering the prior ratings of  users, on average most users prefer equal levels of diversity and similarity. 
Figure~\ref{fig:histograms}.f shows the histogram of heuristic risk is normally distributed and skewed to the right. This suggests heuristic risk is relatively low among users and that  most users are risk-averse, and take less chances with the unpopular items. This is reasonable, since it also supports the long-tail distribution of the popularity vs item demand curve. 
Figure~\ref{fig:histograms}.g --Figure~\ref{fig:histograms}.i show alternative risk-measures. h should be removed. 
\begin{figure*}[htb]
\centering
\subfigure[HistogramNItemofoTrainNRatings]{
\includegraphics[width=0.3\textwidth]{Figures/Histograms/HistogramNItemofoTrainNRatings.pdf} }
%\subfigure[HistogramofoTrainEntropyPop]{
%\includegraphics[width=0.3\textwidth]{Figures/Histograms/HistogramofoTrainEntropyPop.pdf} }
%\subfigure[HistogramofoTrainGini]{
%\includegraphics[width=0.3\textwidth]{Figures/Histograms/HistogramofoTrainGini.pdf}}
%\subfigure[HistogramofoTrainGiniPop]{
%\includegraphics[width=0.3\textwidth]{Figures/Histograms/HistogramofoTrainGiniPop.pdf}}
%\subfigure[HistogramofoTrainGiniSecond]{
%\includegraphics[width=0.3\textwidth]{Figures/Histograms/HistogramofoTrainGiniSecond.pdf}}
\subfigure[HistogramofoTrainNLTItems]{
\includegraphics[width=0.3\textwidth]{Figures/Histograms/HistogramofoTrainNLTItems.pdf}}
\subfigure[HistogramofoTrainNorNLTItems]{
\includegraphics[width=0.3\textwidth]{Figures/Histograms/HistogramofoTrainNorNLTItems.pdf}}
\subfigure[HistogramofoTrainNRatings]{
\includegraphics[width=0.3\textwidth]{Figures/Histograms/HistogramofoTrainNRatings.pdf}}
%\subfigure[HistogramofoTrainVmr]{
%\includegraphics[width=0.3\textwidth]{Figures/Histograms/HistogramofoTrainVmr.pdf}}
\subfigure[Histogramofrho]{
\includegraphics[width=0.3\textwidth]{Figures/Histograms/Histogramofrho.pdf}}
\subfigure[Histogramoftheta]{
\includegraphics[width=0.3\textwidth]{Figures/Histograms/Histogramoftheta.pdf}}
\subfigure[HistogramofthetaIDFN]{
\includegraphics[width=0.3\textwidth]{Figures/Histograms/HistogramofthetaIDFN.pdf}}
\subfigure[HistogramofthetaIDF]{
\includegraphics[width=0.3\textwidth]{Figures/Histograms/HistogramofthetaIDF.pdf}}
%\subfigure[HistogramofoTrainSkewPop]{
%\includegraphics[width=0.3\textwidth]{Figures/Histograms/HistogramofoTrainSkewPop.pdf}}
\subfigure[HistogramofoTrainSkewPop3]{
\includegraphics[width=0.3\textwidth]{Figures/Histograms/HistogramofoTrainSkewPop3.pdf}}

\caption{histograms}
\label{fig:histograms}
\end{figure*}

\subsection{Recommendation performance across users}
In this section we evaluate recommendation performance across users.  In Figures~\ref{fig:metricchanges-oTrainNorNLTItems} -- \ref{fig:metricchanges-rho} we consider K=15, and report the performance metrics as different consumer modelling measures are varied.

\textbf{Risk Degree}
Figure~\ref{fig:metricchanges-theta} depicts the changes across various metrics change as heuristic risk $\theta_u^h$ increases. Note that higher $\theta_u^h$ corresponds to risk-loving users that are  more willing to take chances with less popular items. Therefore, as $\theta_u^h$ increases we expect more long-tail items to be offered , and LTaccuracy to be increasing.  This is confirmed in Figure~\ref{fig:metricchanges-theta}.a, where LTAccuracy increases as $\theta_u^h$ increases (true for all of our methods). Regarding our baselines,  they have not been designed with regard to this measure, and are relatively stable, e.g., MF is independent of this measure. However, we note that long-tail accuracy of wlim decreases as users become more risk-loving.

Moreover, as there is a system trade-off between relevance and long tail promotion,  we expect relevance to be non-increasing as  $\theta_u^h$ increases. Figure~\ref{fig:metricchanges-theta}.c plots relevance vs $\theta_u^h$, where we observe that as  $\theta_u^h$ increases, the relevance of items offered by our method decreases. Particularly,  risk-averse users are offered more relevant items, while  risk-loving users are offered less  relevant items(true for other variants of our method except thetaIDFN). Regarding our baselines, the relevance of items offered is either relatively constant, increasing,  or with fluctuations. E.g.,  as $\theta_u^h$ increases, the relevance of items offered by wlim also increases, which is intuitively incorrect. 

In Figure~\ref{fig:metricchanges-thetaIDFN}, thetaIDfN is used as an alternative risk measure. Figure~\ref{fig:metricchanges-thetaIDFN}.a shows the LTAccuracy, where wlim is decreasing and other methods are relativity stable.  Figure~\ref{fig:metricchanges-thetaIDFN}.c, shows that as this measure increases, relevance of items offered by our method is relatively stable, while our baselines methods increase, which is incorrect.

\textcolor{red}{what about diversity, is it reasonable to expect it to be correlated with theta? } diversity, shown in Figure~\ref{fig:metricchanges-theta}.b. 

\textbf{Focusing Degree} Figure~\ref{fig:metricchanges-rho} considers the focusing degree $\rho$. In Figure~\ref{fig:metricchanges-rho}.c, we observe that as $\rho$ increases, the relevance of items offered to users increases and eventually saturates. However, for all methods excluding our method, the point of saturation is $\rho \approx 0.25$, while for our method it is $\rho \approx 0.6$. Due to the trade-off between diversity and relevance, we see the opposite trend for the diversity measure, in Figure~\ref{fig:metricchanges-rho}.b.  Anything about LTAccuracy? 

\begin{figure*}[htb]
\centering
\subfigure[LTAccuracy]{
\includegraphics[width=0.15\textwidth]{Figures/metricChangesAcrossUsers15/oTrainNorNLTItems/meanLTAccuracyDictoveroTrainNorNLTItems.pdf} 
}
\subfigure[Diversity]{
\includegraphics[width=0.15\textwidth]{Figures/metricChangesAcrossUsers15/oTrainNorNLTItems/meandiversityDictoveroTrainNorNLTItems.pdf} 
}
\subfigure[Relevance]{
\includegraphics[width=0.15\textwidth]{Figures/metricChangesAcrossUsers15/oTrainNorNLTItems/meanrelevanceDictoveroTrainNorNLTItems.pdf}
}
\subfigure[Recall]{
\includegraphics[width=0.15\textwidth]{Figures/metricChangesAcrossUsers15/oTrainNorNLTItems/meanrecallDictoveroTrainNorNLTItems.pdf} 
}
\subfigure[HistogramofoTrainNorNLTItems]{
\includegraphics[width=0.15\textwidth]{Figures/Histograms/HistogramofoTrainNorNLTItems.pdf}}
\caption{changes across users, $K=15$}
\label{fig:metricchanges-oTrainNorNLTItems}
\end{figure*}




\begin{figure*}[htb]
\centering
\subfigure[LTAccuracy]{
\includegraphics[width=0.15\textwidth]{Figures/metricChangesAcrossUsers15/oTrainSkewPop3/meanLTAccuracyDictoveroTrainSkewPop3.pdf} 
}
\subfigure[Diversity]{
\includegraphics[width=0.15\textwidth]{Figures/metricChangesAcrossUsers15/oTrainSkewPop3/meandiversityDictoveroTrainSkewPop3.pdf} 
}
\subfigure[Relevance]{
\includegraphics[width=0.15\textwidth]{Figures/metricChangesAcrossUsers15/oTrainSkewPop3/meanrelevanceDictoveroTrainSkewPop3.pdf}
}
\subfigure[Recall]{
\includegraphics[width=0.15\textwidth]{Figures/metricChangesAcrossUsers15/oTrainSkewPop3/meanrecallDictoveroTrainSkewPop3.pdf} 
}
\subfigure[HistogramofoTrainSkewPop3]{
\includegraphics[width=0.15\textwidth]{Figures/Histograms/HistogramofoTrainSkewPop3.pdf}}
\caption{changes across users, $K=15$}
\label{fig:metricchanges-oTrainSkewPop3}
\end{figure*}




\begin{figure*}[htb]
\centering
\subfigure[LTAccuracy]{
\includegraphics[width=0.15\textwidth]{Figures/metricChangesAcrossUsers15/theta/meanLTAccuracyDictovertheta.pdf} 
}
\subfigure[Diversity]{
\includegraphics[width=0.15\textwidth]{Figures/metricChangesAcrossUsers15/theta/meandiversityDictovertheta.pdf} 
}
\subfigure[Relevance]{
\includegraphics[width=0.15\textwidth]{Figures/metricChangesAcrossUsers15/theta/meanrelevanceDictovertheta.pdf} 
}
\subfigure[Recall]{
\includegraphics[width=0.15\textwidth]{Figures/metricChangesAcrossUsers15/theta/meanrecallDictovertheta.pdf} 
}
\subfigure[Histogramoftheta]{
\includegraphics[width=0.15\textwidth]{Figures/Histograms/Histogramoftheta.pdf}}
\caption{changes across users, $K=15$}
\label{fig:metricchanges-theta}
\end{figure*}



\begin{figure*}[htb]
\centering
\subfigure[LTAccuracy]{
\includegraphics[width=0.15\textwidth]{Figures/metricChangesAcrossUsers15/thetaIDFN/meanLTAccuracyDictoverthetaIDFN.pdf} 
}
\subfigure[Diversity]{
\includegraphics[width=0.15\textwidth]{Figures/metricChangesAcrossUsers15/thetaIDFN/meandiversityDictoverthetaIDFN.pdf} 
}
\subfigure[Relevance]{
\includegraphics[width=0.15\textwidth]{Figures/metricChangesAcrossUsers15/thetaIDFN/meanrelevanceDictoverthetaIDFN.pdf} 
}
\subfigure[Recall]{
\includegraphics[width=0.15\textwidth]{Figures/metricChangesAcrossUsers15/thetaIDFN/meanrecallDictoverthetaIDFN.pdf} 
}
\subfigure[HistogramofthetaIDFN]{
\includegraphics[width=0.15\textwidth]{Figures/Histograms/HistogramofthetaIDFN.pdf}}
\caption{changes across users, $K=15$}
\label{fig:metricchanges-thetaIDFN}
\end{figure*}


\begin{figure*}[htb]
\centering
\subfigure[LTAccuracy]{
\includegraphics[width=0.15\textwidth]{Figures/metricChangesAcrossUsers15/thetaIDF/meanLTAccuracyDictoverthetaIDF.pdf} 
}
\subfigure[Diversity]{
\includegraphics[width=0.15\textwidth]{Figures/metricChangesAcrossUsers15/thetaIDF/meandiversityDictoverthetaIDF.pdf} 
}
\subfigure[Relevance]{
\includegraphics[width=0.15\textwidth]{Figures/metricChangesAcrossUsers15/thetaIDF/meanrelevanceDictoverthetaIDF.pdf} 
}
\subfigure[Recall]{
\includegraphics[width=0.15\textwidth]{Figures/metricChangesAcrossUsers15/thetaIDF/meanrecallDictoverthetaIDF.pdf} 
}
\subfigure[HistogramofthetaIDF]{
\includegraphics[width=0.15\textwidth]{Figures/Histograms/HistogramofthetaIDF.pdf}}
\caption{changes across users, $K=15$}
\label{fig:metricchanges-thetaIDF}
\end{figure*}


\begin{figure*}[htb]
\centering
\subfigure[LTAccuracy]{
\includegraphics[width=0.15\textwidth]{Figures/metricChangesAcrossUsers15/oTrainNRatings/meanLTAccuracyDictoveroTrainNRatings.pdf} 
}
\subfigure[Diversity]{
\includegraphics[width=0.15\textwidth]{Figures/metricChangesAcrossUsers15/oTrainNRatings/meandiversityDictoveroTrainNRatings.pdf} 
}
\subfigure[Relevance]{
\includegraphics[width=0.15\textwidth]{Figures/metricChangesAcrossUsers15/oTrainNRatings/meanrelevanceDictoveroTrainNRatings.pdf}
}
\subfigure[Recall]{
\includegraphics[width=0.15\textwidth]{Figures/metricChangesAcrossUsers15/oTrainNRatings/meanrecallDictoveroTrainNRatings.pdf} 
}
\subfigure[HistogramofoTrainNRatings]{
\includegraphics[width=0.15\textwidth]{Figures/Histograms/HistogramofoTrainNRatings.pdf}}
\caption{changes across users, $K=15$}
\label{fig:metricchanges-oTrainNRatings}
\end{figure*}


  
\begin{figure*}[htb]
\centering
\subfigure[LTAccuracy]{
\includegraphics[width=0.15\textwidth]{Figures/metricChangesAcrossUsers15/rho/meanLTAccuracyDictoverrho.pdf} 
}
\subfigure[Diversity]{
\includegraphics[width=0.15\textwidth]{Figures/metricChangesAcrossUsers15/rho/meandiversityDictoverrho.pdf} 
}
\subfigure[Relevance]{
\includegraphics[width=0.15\textwidth]{Figures/metricChangesAcrossUsers15/rho/meanrelevanceDictoverrho.pdf}
}
\subfigure[Recall]{
\includegraphics[width=0.15\textwidth]{Figures/metricChangesAcrossUsers15/rho/meanrecallDictoverrho.pdf} 
}
\subfigure[Histogramofrho]{
\includegraphics[width=0.15\textwidth]{Figures/Histograms/Histogramofrho.pdf}}
\caption{changes across users, $K=15$}
\label{fig:metricchanges-rho}
\end{figure*}


\subsection{Effect of risk ordering} Figures~\ref{fig:riskorderingeffect-NorNLT}--\ref{fig:riskorderingeffect-oTrainNRatings} examine the effect of making recommendations to users in order of increasing risk-degree  compared to randomly selecting users and recommending items. Figure~\ref{fig:riskorderingeffect-Theta} considers heuristic risk as the measure of risk-degree. Figures~\ref{fig:riskorderingeffect-Theta}.a --~\ref{fig:riskorderingeffect-Theta}.d show that by sorting users in order of increasing heuristic risk, we achieve better coverage, gini, long tail accuracy, and diversity.  However, this ordering results in a loss of relevance, as depicted by Figure~\ref{fig:riskorderingeffect-Theta}.e. The reason is that our algorithm sacrifices the relevance of movies offered to increase the overall coverage of the system. Our risk ordering, however, is devised so that the right group of users are targeted for this objective. Looking back at Figure~ref{fig:metricchanges-thetaIDF}.c, we can observe that indeed more risk-averse users 	are offered more relevant items, and the risk-loving users are offered the long-tail items that increase the coverage, gini of the system. Similar performance trends are observed for the other risk measures: NorNLT Figure~\ref{fig:riskorderingeffect-NorNLT}, Skewpop3 Figures~\ref{fig:riskorderingeffect-SkewPop3}, and ThetaIDFN* Figure~\ref{fig:riskorderingeffect-ThetaIDFN} . For the cases where we don't normalize the risk measure to account for the number of ratings (ThetaIDF Figure~\ref{fig:riskorderingeffect-ThetaIDF},oTrainNRatings Figure~\ref{fig:riskorderingeffect-oTrainNRatings}) we obtain lower diversity and relevance.

\begin{figure*}[tb]
\centering
\subfigure[Coverage]{
\includegraphics[width=0.15\textwidth]{Figures/NoRiskOrderingFigures/NorNLT/noRiskOrderingNorNLTvslazyGreedyNorNLTcoverageoverK.pdf} % 580
}
\subfigure[Gini]{
\includegraphics[width=0.15\textwidth]{Figures/NoRiskOrderingFigures/NorNLT/noRiskOrderingNorNLTvslazyGreedyNorNLTginioverK.pdf} % 577
}
\subfigure[LTAccuracy]{
\includegraphics[width=0.15\textwidth]{Figures/NoRiskOrderingFigures/NorNLT/noRiskOrderingNorNLTvslazyGreedyNorNLTLTAccuracyoverK.pdf} % 578
}
\subfigure[Diversity]{
\includegraphics[width=0.15\textwidth]{Figures/NoRiskOrderingFigures/NorNLT/noRiskOrderingNorNLTvslazyGreedyNorNLTdiversityoverK.pdf} % 579
}



\subfigure[Relevance]{
\includegraphics[width=0.15\textwidth]{Figures/NoRiskOrderingFigures/NorNLT/noRiskOrderingNorNLTvslazyGreedyNorNLTrelevanceoverK.pdf} % 577
}
\subfigure[Recall]{
\includegraphics[width=0.15\textwidth]{Figures/NoRiskOrderingFigures/NorNLT/noRiskOrderingNorNLTvslazyGreedyNorNLTrecalloverK.pdf} % 577
}
\subfigure[HistogramofoTrainNorNLTItems]{
\includegraphics[width=0.15\textwidth]{Figures/Histograms/HistogramofoTrainNorNLTItems.pdf}}
\caption{Effect of sorting consumers by risk measure vs randomly selecting users}
\label{fig:riskorderingeffect-NorNLT}
\end{figure*}


\begin{figure*}[htb]
\centering
\subfigure[Coverage]{
\includegraphics[width=0.15\textwidth]{Figures/NoRiskOrderingFigures/SkewPop3/noRiskOrderingSkewPop3vslazyGreedySkewPop3coverageoverK.pdf} % 580
}
\subfigure[Gini]{
\includegraphics[width=0.15\textwidth]{Figures/NoRiskOrderingFigures/SkewPop3/noRiskOrderingSkewPop3vslazyGreedySkewPop3ginioverK.pdf} % 577
}
\subfigure[LTAccuracy]{
\includegraphics[width=0.15\textwidth]{Figures/NoRiskOrderingFigures/SkewPop3/noRiskOrderingSkewPop3vslazyGreedySkewPop3LTAccuracyoverK.pdf} % 578
}
\subfigure[Diversity]{
\includegraphics[width=0.15\textwidth]{Figures/NoRiskOrderingFigures/SkewPop3/noRiskOrderingSkewPop3vslazyGreedySkewPop3diversityoverK.pdf} % 579
}



\subfigure[Relevance]{
\includegraphics[width=0.15\textwidth]{Figures/NoRiskOrderingFigures/SkewPop3/noRiskOrderingSkewPop3vslazyGreedySkewPop3relevanceoverK.pdf} % 577
}
\subfigure[Recall]{
\includegraphics[width=0.15\textwidth]{Figures/NoRiskOrderingFigures/SkewPop3/noRiskOrderingSkewPop3vslazyGreedySkewPop3recalloverK.pdf} % 577
}
\subfigure[HistogramofoTrainSkewPop3]{
\includegraphics[width=0.15\textwidth]{Figures/Histograms/HistogramofoTrainSkewPop3.pdf}}
\caption{Effect of sorting consumers by risk measure vs randomly selecting users}
\label{fig:riskorderingeffect-SkewPop3}
\end{figure*}



\begin{figure*}[htb]
\centering
\subfigure[Coverage]{
\includegraphics[width=0.15\textwidth]{Figures/NoRiskOrderingFigures/Theta/noRiskOrderingThetavslazyGreedyThetacoverageoverK.pdf} % 580
}
\subfigure[Gini]{
\includegraphics[width=0.15\textwidth]{Figures/NoRiskOrderingFigures/Theta/noRiskOrderingThetavslazyGreedyThetaginioverK.pdf} % 577
}
\subfigure[LTAccuracy]{
\includegraphics[width=0.15\textwidth]{Figures/NoRiskOrderingFigures/Theta/noRiskOrderingThetavslazyGreedyThetaLTAccuracyoverK.pdf} % 578
}
\subfigure[Diversity]{
\includegraphics[width=0.15\textwidth]{Figures/NoRiskOrderingFigures/Theta/noRiskOrderingThetavslazyGreedyThetadiversityoverK.pdf} % 579
}




\subfigure[Relevance]{
\includegraphics[width=0.15\textwidth]{Figures/NoRiskOrderingFigures/Theta/noRiskOrderingThetavslazyGreedyThetarelevanceoverK.pdf} % 577
}
\subfigure[Recall]{
\includegraphics[width=0.15\textwidth]{Figures/NoRiskOrderingFigures/Theta/noRiskOrderingThetavslazyGreedyThetarecalloverK.pdf} % 577
}
\subfigure[Histogramoftheta]{
\includegraphics[width=0.15\textwidth]{Figures/Histograms/Histogramoftheta.pdf}}
\caption{Effect of sorting consumers by risk measure vs randomly selecting users}
\label{fig:riskorderingeffect-Theta}
\end{figure*}


\begin{figure*}[htb]
\centering
\subfigure[Coverage]{
\includegraphics[width=0.15\textwidth]{Figures/NoRiskOrderingFigures/ThetaIDFN/noRiskOrderingThetaIDFNvslazyGreedyThetaIDFNcoverageoverK.pdf} % 580
}
\subfigure[Gini]{
\includegraphics[width=0.15\textwidth]{Figures/NoRiskOrderingFigures/ThetaIDFN/noRiskOrderingThetaIDFNvslazyGreedyThetaIDFNginioverK.pdf} % 577
}
\subfigure[LTAccuracy]{
\includegraphics[width=0.15\textwidth]{Figures/NoRiskOrderingFigures/ThetaIDFN/noRiskOrderingThetaIDFNvslazyGreedyThetaIDFNLTAccuracyoverK.pdf} % 578
}
\subfigure[Diversity]{
\includegraphics[width=0.15\textwidth]{Figures/NoRiskOrderingFigures/ThetaIDFN/noRiskOrderingThetaIDFNvslazyGreedyThetaIDFNdiversityoverK.pdf} % 579
}



\subfigure[Relevance]{
\includegraphics[width=0.15\textwidth]{Figures/NoRiskOrderingFigures/ThetaIDFN/noRiskOrderingThetaIDFNvslazyGreedyThetaIDFNrelevanceoverK.pdf} % 577
}
\subfigure[Recall]{
\includegraphics[width=0.15\textwidth]{Figures/NoRiskOrderingFigures/ThetaIDFN/noRiskOrderingThetaIDFNvslazyGreedyThetaIDFNrecalloverK.pdf} % 577
}
\subfigure[HistogramofthetaIDFN]{
\includegraphics[width=0.15\textwidth]{Figures/Histograms/HistogramofthetaIDFN.pdf}}
\caption{Effect of sorting consumers by risk measure vs randomly selecting users}
\label{fig:riskorderingeffect-ThetaIDFN}
\end{figure*}


\begin{figure*}[htb]
\centering
\subfigure[Coverage]{
\includegraphics[width=0.15\textwidth]{Figures/NoRiskOrderingFigures/ThetaIDF/noRiskOrderingThetaIDFvslazyGreedyThetaIDFcoverageoverK.pdf} % 580
}
\subfigure[Gini]{
\includegraphics[width=0.15\textwidth]{Figures/NoRiskOrderingFigures/ThetaIDF/noRiskOrderingThetaIDFvslazyGreedyThetaIDFginioverK.pdf} % 577
}
\subfigure[LTAccuracy]{
\includegraphics[width=0.15\textwidth]{Figures/NoRiskOrderingFigures/ThetaIDF/noRiskOrderingThetaIDFvslazyGreedyThetaIDFLTAccuracyoverK.pdf} % 578
}
\subfigure[Diversity]{
\includegraphics[width=0.15\textwidth]{Figures/NoRiskOrderingFigures/ThetaIDF/noRiskOrderingThetaIDFvslazyGreedyThetaIDFdiversityoverK.pdf} % 579
}



\subfigure[Relevance]{
\includegraphics[width=0.15\textwidth]{Figures/NoRiskOrderingFigures/ThetaIDF/noRiskOrderingThetaIDFvslazyGreedyThetaIDFrelevanceoverK.pdf} % 577
}
\subfigure[Recall]{
\includegraphics[width=0.15\textwidth]{Figures/NoRiskOrderingFigures/ThetaIDF/noRiskOrderingThetaIDFvslazyGreedyThetaIDFrecalloverK.pdf} % 577
}
\subfigure[HistogramofthetaIDF]{
\includegraphics[width=0.15\textwidth]{Figures/Histograms/HistogramofthetaIDF.pdf}}
\caption{Effect of sorting consumers by risk measure vs randomly selecting users}
\label{fig:riskorderingeffect-ThetaIDF}
\end{figure*}


\begin{figure*}[htb]
\centering
\subfigure[Coverage]{
\includegraphics[width=0.15\textwidth]{Figures/NoRiskOrderingFigures/NRatings/noRiskOrderingNRatingsvslazyGreedyNRatingscoverageoverK.pdf} % 580
}
\subfigure[Gini]{
\includegraphics[width=0.15\textwidth]{Figures/NoRiskOrderingFigures/NRatings/noRiskOrderingNRatingsvslazyGreedyNRatingsginioverK.pdf} % 577
}
\subfigure[LTAccuracy]{
\includegraphics[width=0.15\textwidth]{Figures/NoRiskOrderingFigures/NRatings/noRiskOrderingNRatingsvslazyGreedyNRatingsLTAccuracyoverK.pdf} % 578
}
\subfigure[Diversity]{
\includegraphics[width=0.15\textwidth]{Figures/NoRiskOrderingFigures/NRatings/noRiskOrderingNRatingsvslazyGreedyNRatingsdiversityoverK.pdf} % 579
}


\subfigure[Relevance]{
\includegraphics[width=0.15\textwidth]{Figures/NoRiskOrderingFigures/NRatings/noRiskOrderingNRatingsvslazyGreedyNRatingsrelevanceoverK.pdf} % 577
}
\subfigure[Recall]{
\includegraphics[width=0.15\textwidth]{Figures/NoRiskOrderingFigures/NRatings/noRiskOrderingNRatingsvslazyGreedyNRatingsrecalloverK.pdf} % 577
}
\subfigure[HistogramofoTrainNRatings]{
\includegraphics[width=0.15\textwidth]{Figures/Histograms/HistogramofoTrainNRatings.pdf}}
\caption{Effect of sorting consumers by risk measure vs randomly selecting users}
\label{fig:riskorderingeffect-oTrainNRatings}
\end{figure*}


%^^^^^^^^^^^^^^^^^^^^^^^^^^^^^^^^^^^^^^^^^^^^^^^^^^^^^^^^^^^^^^^^^^^^^^^^^^^^^^^^^^^^^^^^^^^^^^^^^^^^^^6


\subsection{Top-K Recommendation performance evaluation}
Figure~\ref{fig:metrics} plots Top-K performance metrics consisting of coverage, gini, long-tail accuracy, diversity, and relevance as K is varied. We compare different variants of our algorithm (denoted as lazy greedy in all plots), traditional matrix factorization (MF) and four variants of our baseline, wlim. 
Figure~\ref{fig:metrics}.a shows coverage, where most of our methods achieve a coverage of 1 at K=5 (heuristic risk at K=10). wlim is lower. 
Figure~\ref{fig:metrics}.b, shows gini where a lower gini score represents a more balanced recommendation set(\textcolor{red}{can we say this for sure, or use entropy?}). All variants of our method achieve a lower gini coefficient. However, among the the baselines, wlim  has the lowest gini coefficient. 
Figure~\ref{fig:metrics}.c shows LTAccuracy performance.  Even though wlim achieves the best overall LTAccuracy, it has lower coverage and a smaller gini coefficient. 
Figure~\ref{fig:metrics}.d shows diversity  where  wlim is closely followed by our methods, then MF and other varients of wlim. 
Figure~\ref{fig:metrics}.e, shows relevance, currently not scaled.  MF has the best performance, then our method, variants of wlim. 

\begin{figure*}[htb]
\centering
\subfigure[Coverage]{
\includegraphics[width=0.45\textwidth]{Figures/metrics/coverageoverK.pdf} % 580
}
\subfigure[Gini]{
\includegraphics[width=0.45\textwidth]{Figures/metrics/ginioverK.pdf} % 577
}
\subfigure[LTAccuracy]{
\includegraphics[width=0.45\textwidth]{Figures/metrics/LTAccuracyoverK.pdf} % 578
}
\subfigure[Diversity]{
\includegraphics[width=0.45\textwidth]{Figures/metrics/diversityoverK.pdf} % 579
}
\subfigure[Relevance]{
\includegraphics[width=0.45\textwidth]{Figures/metrics/relevanceoverK.pdf} % 577
}
\subfigure[Recall]{
\includegraphics[width=0.45\textwidth]{Figures/metrics/recalloverK.pdf} % 577
}
\caption{Top-$K$ recommendation performance metrics vs $K$.}
\label{fig:metrics}
\end{figure*}
\fi
